# Supplementary material for: Trade When Opportunity Comes: Price Movement Forecasting via Locality-Aware Attention and Iterative Refinement Labeling
Source: arXiv:2107.11972 source file (2024-07-10)
Supplement: Supplementary file 1 [file Appendix.tex]

\subsection{Experiments settings}
\label{appendix:experiments-settings}

% \subsubsection{Experiment Environment}
% \ 
% \newline
% \indent We conduct all experiments with the following setting:
% \begin{enumerate}
%     \item[$\blacktriangleright$] Operating system: Ubuntu 5.4.0-6ubuntu1~16.04.12
%     \item[$\blacktriangleright$] CPU: Intel(R) Xeon(R) Gold 6230 CPU @ 2.10GHz
%     \item[$\blacktriangleright$] Software versions: Python 3.7; Numpy 1.19.2; Pandas 1.0.5; Lightgbm 2.2.3; scikit-learn 0.23.2; hnswlib 0.4.0; Scipy 1.5.2; Metric-learn  0.6.2
% \end{enumerate}

\subsubsection{Parameter Settings}
\ 
\newline
\indent For the reproducibility of our proposed methods, we describe the parameter settings in detail here.

\begin{table}[hbp]
    \centering
    \small
    \caption{Hyper-parameters for each ETF}
    \vspace{-0.2cm}
    \scalebox{0.9}{
    \begin{tabular}{c|cccccc}
    \toprule
        ETF & K-NN/R-NN & K & R & Times & Ratio & Ensemble\\
    \midrule
    \multicolumn{7}{c}{Positive Cases}\\
    \midrule
        159915.SZ & K-NN & 150 & - & 7 & 0.05 & vote \\
        512480.SH & R-NN & 90 & 100 & 9 & 0.04 & vote \\
        512880.SH & R-NN & 150 & 50 & 7 & 0.07 & vote \\
        515050.SH & K-NN & 120 & - & 9 & 0.05 & vote \\
    \midrule
    \multicolumn{7}{c}{Negative Cases}\\
    \midrule
        159915.SZ & K-NN & 100 & - & 9 & 0.07 & vote \\
        512480.SH & R-NN & 150 & 30 & 9 & 0.03 & vote \\
        512880.SH & K-NN & 150 & - & 9 & 0.10 & vote \\
        515050.SH & K-NN & 150 & - & 7 & 0.10 & vote \\
    \midrule
    \end{tabular}
    \label{tab:hyper-parameters}
    }
\end{table}

% \noindent
% \textbf{Timespan}:
% \begin{itemize}
%     \item Training set: Jan. 1, 2020 to Apr. 17, 2020 
%     \item Validation set: Apr. 20, 2020 to May. 29, 2020 
%     \item Testing set: May. 30, 2020 to Jul. 6, 2020 
% \end{itemize}

% \noindent
% \textbf{Metric Learning}: Sparse High-Dimensional Metric Learning (SDML)

% \noindent
% \textbf{HNSW}: The parameter $ef$ is set to $10 \times K$. The maximum number of outgoing connections in the graph is fixed as 16.

% \noindent
% \textbf{Lightgbm}: Boosting type is set to 'gbdt' and the objective is 'binary'. Other parameters are set to the default recommended ones for a fair comparison.

\begin{table*}[htp]
    \centering
    \caption{Quantitative comparisons among different methods on 515050.SH ETF. 
    % The first part of the table compares the quality of the signals generated by a threshold. The second part of the table compares the quality of the most convinced 1000 signals of different models on the test set. Due to the ensemble algorithm in Bi-level Labeling, it is hard to control the number of the output signals, so we leave out the Bi-Level Labeling method when comparing the top 1000 signals.
    }
    \vspace{-0.4cm}
    \begin{tabular}{cll|cccc}
    \toprule
        \multicolumn{3}{c|}{Methods} & Precision & Win-Loss Ratio & Average Return & \#Transactions \\ 
    \midrule
        \multirow{2}*{Time Series} & \multicolumn{2}{l|}{Ordinary Least Squares} & 55.23$\pm$0.10 & 1.369$\pm$0.001 & 0.00137$\pm$0.00000 & 1000 \\
        & \multicolumn{2}{l|}{ARIMA} & 9.45$\pm$0.00 & 1.006$\pm$0.000 & -0.00008$\pm$0.00000 & 1000 \\
    \midrule
        \multirow{6}*{Machine Learning} & 
        \multicolumn{2}{l|}{AdaBoost} & 38.38$\pm$2.26 & 1.400$\pm$0.077 & 0.00098$\pm$0.00006 & 1000 \\
        & \multicolumn{2}{l|}{Bagging Regressor} & 40.95$\pm$1.19 & 1.465$\pm$0.077 & 0.00104$\pm$0.00001 & 1000 \\
        & \multicolumn{2}{l|}{MLP} & 14.62$\pm$4.37 & 1.131$\pm$0.077 & 0.00029$\pm$0.00015 & 1000 \\
        & \multicolumn{2}{l|}{Ridge} & 46.24$\pm$0.02 & 1.393$\pm$0.002 & 0.00118$\pm$0.00000 & 1000 \\
        & \multicolumn{2}{l|}{Decision Trees} & 20.60$\pm$2.20 & 1.204$\pm$0.030 & 0.00042$\pm$0.00006 & 1000 \\ 
        & \multicolumn{2}{l|}{LightGBM} & 41.21$\pm$1.04 & 1.364$\pm$0.079 & 0.00115$\pm$0.00002 & 1000 \\
    \midrule
        \multirow{3}*{LARA}
         & LA-Attention & \makecell[c]{-} & 56.73$\pm$1.15 & 1.586$\pm$0.099 & \textbf{0.00141}$\pm$0.00003 & 1000 \\
         & \makecell[c]{-} & RA-Labeling & 41.51$\pm$0.78 & 1.362$\pm$0.035 & 0.00116$\pm$0.00001 & 1000 \\
         & LA-Attention & RA-Labeling & \textbf{56.89}$\pm$0.76 & \textbf{1.595}$\pm$0.119 & \textbf{0.00141}$\pm$0.00002 & 1000 \\
    \bottomrule
    \end{tabular}
    
    \label{tab:exp-baseline-ablation-515050}
\end{table*}

\begin{figure*}[htp]
	\centering
	\includegraphics[width=.9\textwidth]{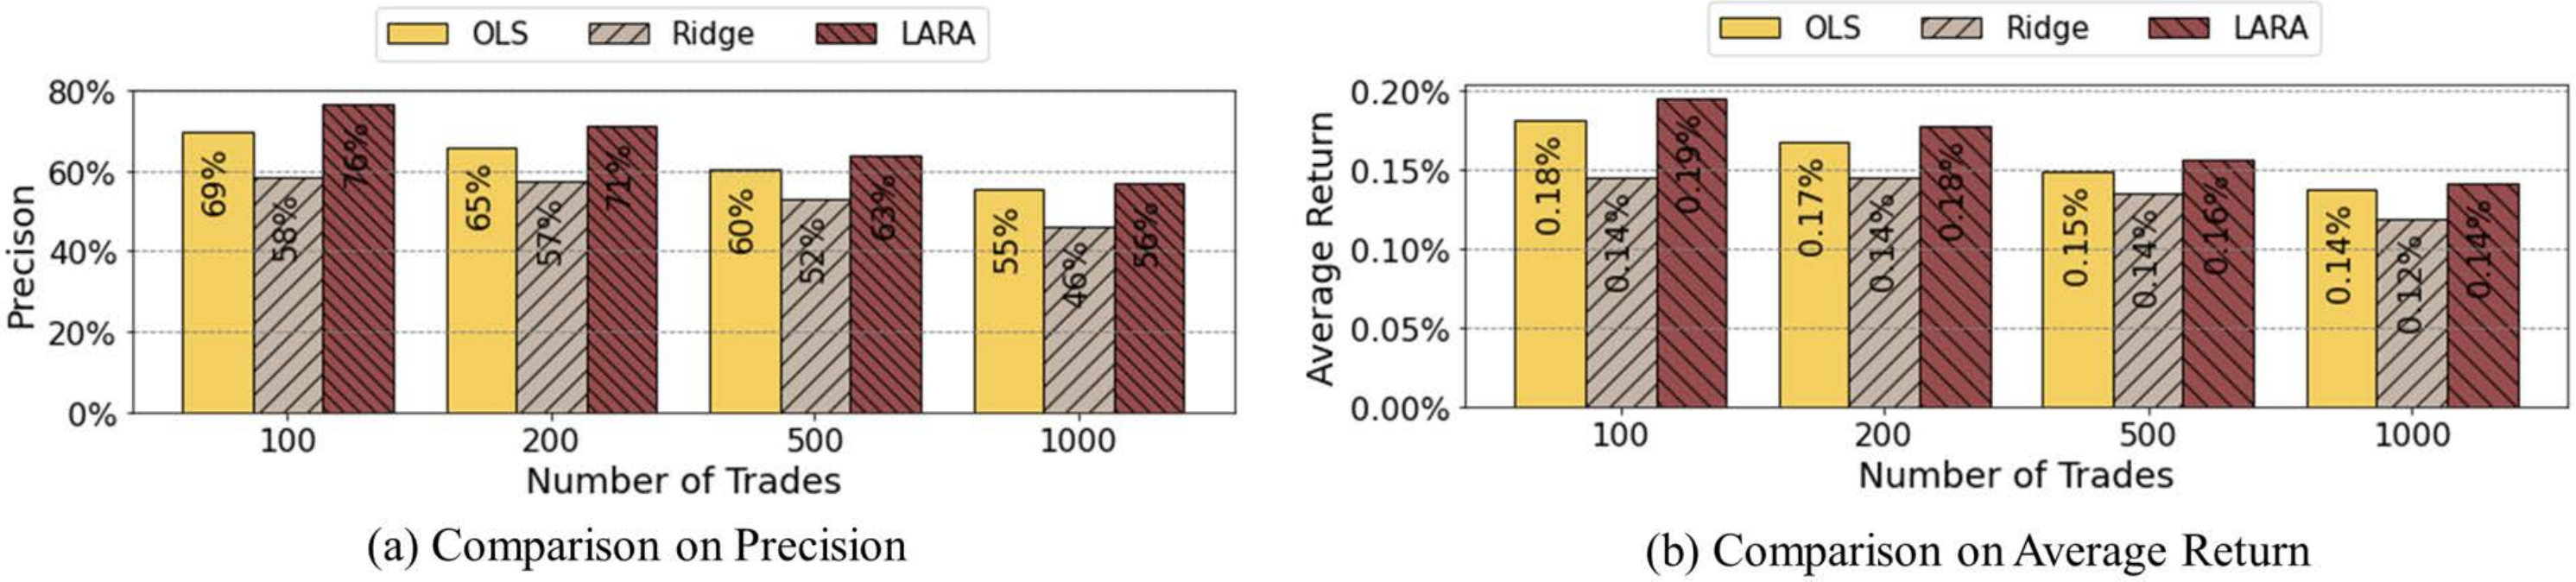}
	\vspace{-0.1cm}
	\caption{Quantitative comparisons among three methods over Precision and Average Return on 515050.SH ETF.}
	\label{fig:trades-diff-515050}
	\vspace{-0.5cm}
\end{figure*}

\noindent
\textbf{Random Seed}: Each experiment is conducted with 5 different seeds as shown below. Positive and negative samples are sampled equally before training, however, these sampled data may not suitable for SDML to search for a positive definite matrix. Hence there are some differences between the seeds for each ETF.
\begin{itemize}
    \item 159915.SZ: 1, 2, 3, 4, 5
    \item 512480.SH: 1, 2, 3, 4, 5
    \item 512880.SH: 1, 2, 8, 9, 11
    \item 515050.SH: 3, 5, 7, 8, 9
\end{itemize}

% \noindent
% \textbf{Search Space} We search for the best hyper-parameters for each ETF on the validation set. And the search space is listed as follow:
% \begin{itemize}
%     \item K-NN/R-NN
%     \item $K \in \{10, 20, 30, ..., 150 \}$
%     \item $R \in \{10, 20, 30, ..., 100 \}$
%     \item RA-Labeling Times $\in \{1, 3, 5, 7, 9\}$
%     \item RA-Labeling Ratio $\in \{0.01, 0.02, 0.03, ..., 0.10\}$
%     \item Ensemble Mode $\in \{vote, \; last\}$
% \end{itemize}

\noindent
\textbf{Hyper-Parameters} After searching, the best parameters of the results we show in this work for K-Neighbor/R-Neighbor, K points, R radius, Two-Side Adaptive Labeling Times, Ratio and Ensemble mode are detailed in Table \ref{tab:hyper-parameters}.

\subsection{An Illustrative Example of LA-Attention}
\label{sec:appendix:example}
To illustrate the effectiveness of our framework, we give a vivid example in Figure \ref{fig:nn-example}. With the large variance samples to simulate the low signal-to-noise ratio financial data, the samples are confused at the junction of two Gaussian Distributions. Training on the whole set given by the blue curve will suffer from a lot of noise, especially near the decision boundary. However, when training only on the \emph{super-class} samples given by our locality-aware label attention algorithm, the prediction boundary of our LARA framework has been pushed further away from the noisy region, leading to a much more convincing prediction. 

\begin{figure}
    \centering
    \includegraphics[width=8cm]{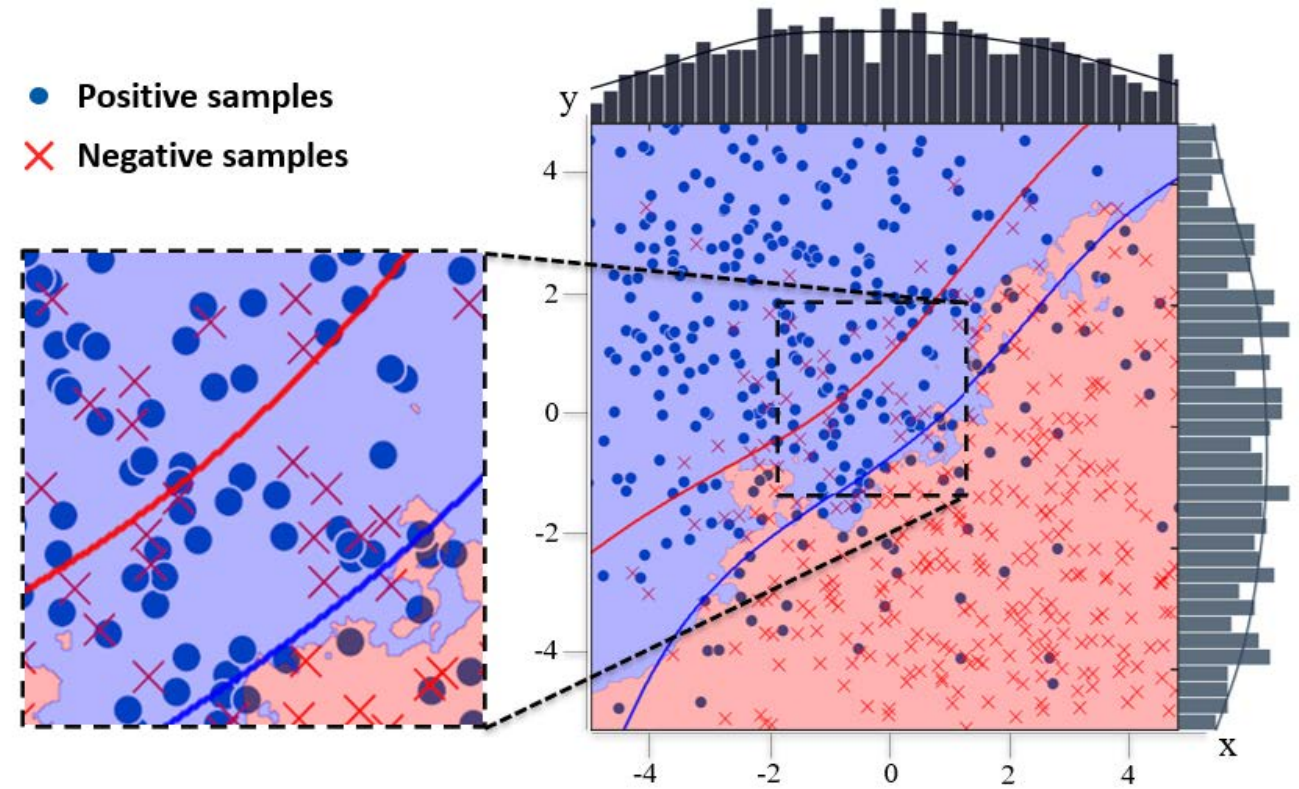}
    \vspace{-0.5cm}
    \caption{An illustrative example of LA-Attention. Randomly sample 400 samples from $\mathcal{N}((-2,2), 8I_2)$ and $\mathcal{N}((2,-2), 8I_2)$ as positive and negative samples respectively. The blue region denotes the super-positive samples given by our LA-Attention. The blue curve is the decision boundary of an SVM classifier training on the whole set, and the red curve is that training only on the super-positive samples.}
    \label{fig:nn-example}
    \vspace{-0.2cm}
\end{figure}

\subsection{Masked Attention Model}
% In \emph{locality-aware attention}, we propose the \emph{masked attention model} to extract the potentially profitable samples by attending to label information of samples in the neighborhood. 
% Specifically, it divides the feature space of training samples into distinct regions with respect to the results of \emph{masked attention model} (Sec. \ref{sec:attention}).
% % and gets potentially profitable samples in the light of the results of \emph{locality-aware attention} (Sec. \ref{sec:attention}). 
% % As a consequence, 
% Therefore, a natural question arises here: 
% \emph{Is masked attention model useful for extracting potentially profitable samples?}

We use an intuitive example to further study the \emph{masked attention} model in Fig. \ref{fig_case}.
Even though the optimal linear classifier (omitting the bias term for convenience) is determined\footnote{This conclusion is intuitive, and the rigorous mathematical proof can refer to \cite{bishop2006pattern}.}, $y = x$ , to classify $\mathcal{N}\left( \left(-2,2\right), 4I_2 \right)$ and $\mathcal{N}\left( \left(2,-2\right), 4I_2 \right)$, the actual classifier built over the sampled datasets deviates from the optimal classifier owing to the insufficient sample size and noise, especially in the middle region where positive and negative samples are mixed together. 
Intuitively, extracting \emph{super-class} samples in the blue and red regions with less noise and training classifiers over them can generate a more robust predictor nearer to the optimal line, which is not susceptible to the \emph{noisy} samples out of the \emph{super-class} area.
In the testing phase, we merely focus on the samples on the \emph{super-class} area, which are easily to be distinguished with respect to the learned predictor.
% in the green region.
Hence, the \emph{locality-aware attention} algorithm, which trains and predicts on the \emph{super-class} samples in the blue and red regions, is more robust to the deviation of the learned decision boundary and generate real profitable signals.
% and deserves further study.

\begin{figure}[htbp]
	\centering
	\includegraphics[width=.40\textwidth]{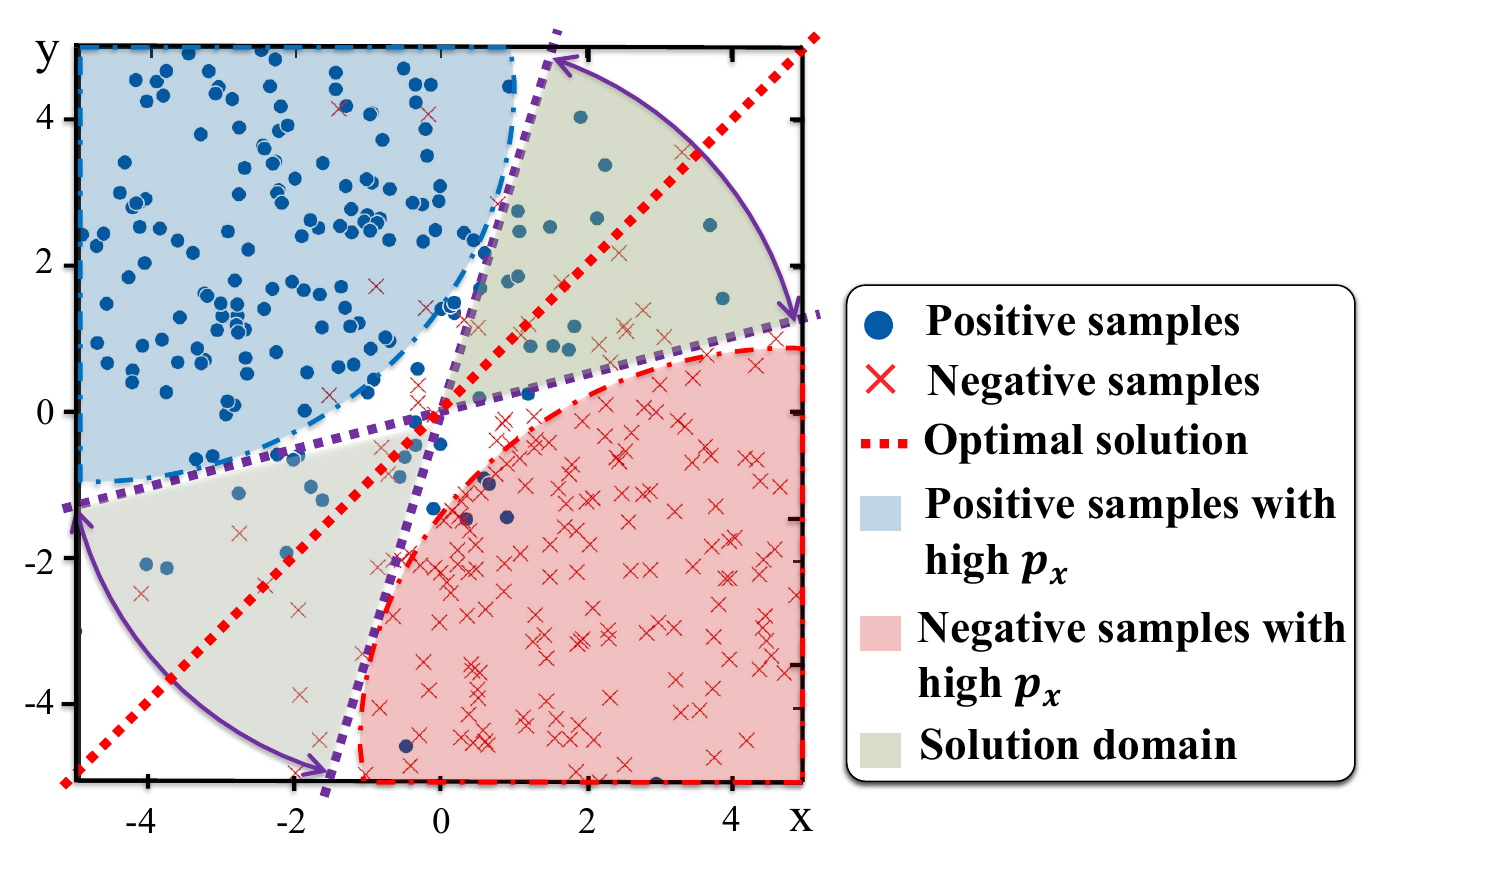}
% 	\vspace{-0.85cm}
	\caption{The didactic example for illustrating \emph{locality-aware attention}. Sample 200 data points from $\mathcal{N}\left( \left(-2,2\right), 4I_2 \right)$ and $\mathcal{N}\left( \left(2,-2\right), 4I_2 \right)$ as positive and negative training samples, respectively. Testing samples are from the same distribution. The blue region (upper left) stands for the super-positive area with less noise. The same for the super-negative area in the red region (lower right). For a linear classifier $y = w \cdot x$, the red dotted line represents the optimal solution and other solutions deviate from the optimal one (mainly located in green) due to insufficient sample size and noise.}
	\label{fig_case}
\end{figure}

\subsection{Additional Experiments}
\label{appendix:experiments}
Here we present the results of another ETF, 515050.SH. As shown in the Table \ref{tab:exp-baseline-ablation-515050}, 
% OLS performs the better in the time-series methods and Ridge Perform better in the machine learning methods. 
Our proposed method outperforms other time series analysis and machine learning methods with the same number of trades.
In addition, our LARA framework outperforms them under the different number of trades shown in Figure \ref{fig:trades-diff-515050}.
