# Supplementary material for: Trade When Opportunity Comes: Price Movement Forecasting via Locality-Aware Attention and Iterative Refinement Labeling
Source: arXiv:2107.11972 source file (2024-07-10)
Supplement: Supplementary file 2 [file Appendix_new.tex]

\section{Experimental Setup}
\subsection{Implementation Details}
\label{sec:implementation}
We adopt the Sparse High-Dimensional Metric Learning (SDML) \cite{qi2009efficient} approach in the \emph{metric learning module}.
We utilize a fast approximate nearest neighbor search method called HNSW \cite{malkov2018efficient} to efficiently implement the K-Neighbor/R-Neighbor algorithm in LA-Attention. 
As introduced in Sec.~\ref{sec:attention}, we consider two kinds of attention weights in LA-Attention: the identical weight $k_i$ to implement the K-Neighbor algorithm and the reciprocal of distance $k_r$ to implement the R-Neighbor algorithm.
Specifically, the HNSW algorithm can be directly adopted in K-Neighbor. As for R-Neighbor, we first query the nearest neighbors with a moderate value of $K$ and then select potentially profitable samples located in a fixed radius $R$. 
The pseudocodes of the K-Neighbor and R-Neighbor algorithms are illustrated in Algorithm~\ref{alg:KNN-RNN-algorithm}.
We employ \emph{LightGBM} \cite{ke2017lightgbm} as the machine learning predictor in the LARA framework since it was reported to be the most commonly-used predictor for financial prediction tasks in several previous works~\cite{zhang2020doubleensemble,xu2020adaptive}.
The combining methods we use in RA-Labeling are \emph{last} and \emph{vote} described in Sec.~\ref{sec:bi-level}. As we study the binary classification problem, we use the~(binary) cross-entropy loss in RA-Labeling.
For LARA, we optimize the hyper-parameters on the validation set using the grid search method. 
\begin{algorithm}[H]
    \caption{K-Neighbor and R-Neighbor algorithm}
    \label{alg:KNN-RNN-algorithm}
    \KwIn{Training data $\left(\mX, \vy\right) \in \mathbb{R}^{N \times d} \times \mathbb{R}^{N}$, the query sample $\vx$, the number of the nearest neighbors $K_N$, and the radius $R_N$.}
  	\KwOut{$\hat{p}_\vx \in \mathbb{R}^N$.}
  	\nonl \textbf{K-Neighbor Algorithm: } \\
  	$\mathcal{N}(\vx)$ = top $K_N$ points with minimum $d_{\mM}(\vz, \vx)$, $\vz \in X$.\\
  	\textbf{Return:} $\hat{p}_\vx = \sum_{\vz_i \in \mathcal{N}(\vx)} y_{z_i} \cdot \frac{k_I(\vz_i, \vx)}{\sum_{\vz_j \in \mathcal{N}(\vx)} k_I(\vz_j, \vx)}$. \\
    % \textbf{Return:} $\hat{p}_x$\\
    \nonl \rule[10pt]{8.0cm}{0.05em}
    \textbf{R-Neighbor Algorithm: } \\
    \setcounter{AlgoLine}{0}
  	$\mathcal{N}_1(\vx)$ = top $K_N$ points with minimum $d_{\mM}(\vz, \vx)$, $\vz \in X$.\\
  	$\mathcal{N}_2(\vx)$ = $\{\vz: \vz \in \mathcal{N}_1(\vx),\; d_{\mM}(\vx, \vz) < R_N \}$. \\
  	\textbf{Return:} $\hat{p}_\vx = \sum_{\vz_i \in \mathcal{N}_2(\vx)} y_{z_i} \cdot \frac{k_R(\vz_i, \vx)}{\sum_{\vz_j \in \mathcal{N}_2(\vx)} k_R(\vz_j, \vx)}$.
    % \textbf{Return:} $\hat{p}_x$\\
\end{algorithm}

\subsection{Hyperparameter Settings}
\label{appendix:experiments-settings}
For the reproducibility of our proposed LARA framework, we describe the hyperparameter settings in detail.
In order to compare different methods fairly, we only carry out a grid search for some selected hyperparameters~(including LA-Attention and RA-Labeling part) on the validation set and the use the default parameters for the base predictor. 
We list the detailed values of $K_N$ in K-Neighbor, $K_N$ and $R_N$ in R-Neighbor, $K$ and $r$ in the RA-Labeling method, and the combination scheme $C$ in Table~\ref{tab:hyper-parameters}.

\setlength{\textfloatsep}{0pt}% Remove \textfloatsep
\begin{table}[htbp]
    \centering
    \caption{Detailed hyperparameters for each dataset.}
    \scalebox{0.85}{
    \begin{tabular}{c|cccccc}
    \toprule
        Data & \begin{tabular}{c} K-Neighbor/ \\ R-Neighbor\end{tabular} & $K_N$ & $R_N$ & $K$ & $r$ & $C$ \\
    \midrule\midrule
    \multicolumn{7}{c}{Long Positions}\\
    \midrule
        Stock  & R-Neighbor & 40 & 60 & 9 & 0.01 & $C_{\text{Vote}}$ \\
        Crypto & R-Neighbor & 40 & 40 & 5 & 0.09 & $C_{\text{Vote}}$ \\
        159915.SZ & K-Neighbor & 150 & - & 7 & 0.05 & $C_{\text{Vote}}$ \\
        512480.SH & R-Neighbor & 90 & 100 & 9 & 0.04 & $C_{\text{Vote}}$ \\
        512880.SH & R-Neighbor & 150 & 50 & 7 & 0.07 & $C_{\text{Vote}}$ \\
        515050.SH & K-Neighbor & 120 & - & 9 & 0.05 & $C_{\text{Vote}}$ \\
    \midrule
    \multicolumn{7}{c}{Short Positions}\\
    \midrule
        159915.SZ & K-Neighbor & 100 & - & 9 & 0.07 & $C_{\text{Vote}}$ \\
        512480.SH & R-Neighbor & 150 & 30 & 9 & 0.03 & $C_{\text{Vote}}$ \\
        512880.SH & K-Neighbor & 150 & - & 9 & 0.10 & $C_{\text{Vote}}$ \\
        515050.SH & K-Neighbor & 150 & - & 7 & 0.10 & $C_{\text{Vote}}$ \\
    \bottomrule
    \end{tabular}
    \label{tab:hyper-parameters}
    }
    % \vspace{2em}
\end{table}

\subsection{Datasets}
The statistics of datasets we used in experiments are summarized in Table~\ref{table_datasets}. We empirically identify that the ratio of positive and negative samples is less than 25\% on ETFs,  highlighting the importance of selecting potentially profitable samples in the noisy financial market. Notice that there are two types of stock data provided in Qlib~\cite{yang2020qlib}, \emph{alpha158} and \emph{alpha360}. These two datasets have different organizational formats. The first \emph{alpha158} is in tabular form, containing 158 factors, while the second \emph{alpha360} is in time-series format, containing 6 attributes and their 60 consecutive time-points. Considering the different data formats and the characteristics of certain models, especially time-series models, we will choose the data format that is suitable for different models. For LARA, due to the nature of the metric learning module, we adopted the \emph{alpha158} dataset.

\subsection{Performance Metrics}
We list the detailed descriptions of each metric as follows:

1) \emph{Precision.} 
In quantitative trading, we care more about samples with positive predictions because these samples can lead us to identify real trading signals. Hence, \textit{precision} is an important criterion for evaluating different models, which can be calculated as $TP / (TP+FP)$, where TP = True Positive and FP = False Positive.

2) \emph{Win-Loss Ratio} is a risk indicator, which is calculated by the ratio of the average mean of winnings to the average mean of losses. It measures the profitability for each of the winnings in excess of that for each of the losses, \ie, $\text{Return of winning} / \text{Return of loss}$.

3) \emph{$\#$Transactions} is an important indicator for high-frequency trading to compare different methods with the same frequency of trades. It is defined as follows: $\# Transactions = \text{The number of trades}$.

4) \emph{Average Return} is a basic and direct index to evaluate the performance of the corresponding strategy in high-frequency trading scenarios. It represents the average return per transaction or the expected profit of each trade, \ie, $\text{Returns} / {\# \text{Transactions}}$.

\begin{table*}[tp]
    \caption{Statistics of datasets used in experiments. \emph{Granularity} indicates the minimum time step of each dataset. $\Delta$ and $\lambda$ denote the time horizon of predictions and the pre-defined threshold, respectively. We also calculate the ratio of positive samples in the long and short positions.}
    \centering
    \scalebox{0.9}{
    \setlength{\tabcolsep}{4pt}
    \begin{tabular}{r|r|cccccc}
    \toprule
        \multicolumn{2}{c|}{Dataset} & \#Instances & Granularity & $\Delta$ & $\lambda$ & Long positions~(Ratio) &  Short positions~(Ratio)  \\
        \midrule
        Stock & CSI300 & 859,230 & 1 day & 1 day & 1E-3 & 409,487 (47.66\%)   & -\footnotemark[2] \\
        \midrule
        Cryptocurrency & BTC/USDT & 10,865,879 & 0.1 sec & 10 secs & 1E-4 & 4,265,413 (39.26\%) & -\footnotemark[2] \\
        \midrule
        \multirow{4}*{ETF} 
        & 159915.SZ & 448,360 & 3 secs & 1 min & 1E-3  & 60,141 (13.41\%) & 58,344 (13.01\%)  \\ 
        & 512480.SH & 433,231 & 3 secs & 1 min & 1E-3  & 99,907 (23.06\%) & 102,967 (23.77\%)\hspace{0.5em} \\
        & 512880.SH & 448,613 & 3 secs & 1 min & 1E-3  & 97,579 (21.75\%) & 99,775 (22.24\%) \\
        & 515050.SH & 459,648 & 3 secs & 1 min & 1E-3  & 53,457 (11.63\%) & 52,399 (11.40\%) \\ 
    \bottomrule
    \end{tabular}
    }
    \label{table_datasets}
\end{table*}

\subsection{Experiments Settings}
All experiments are conducted with the following settings:
\begin{itemize}[leftmargin=14pt]
    \item Operating system: Ubuntu Linux 16.04.7 LTS
    \item CPU: Intel(R) Xeon(R) Silver 4210 CPU @ 2.20GHz
    \item GPU: NVIDIA GP102GL [Tesla P40]
    \item Software versions: Python 3.7; Pytorch 1.9.0+cu102; Numpy 1.21.5; SciPy 1.7.0; Pandas 1.0.5; Scikit-learn 0.23.2; Hnswlib 0.4.0; Metric-learn 0.6.2
\end{itemize}

\begin{table*}[htbp]
    \centering
    \small
    \caption{Quantitative comparisons among different methods on the China's A-share stocks and the cryptocurrency (BTC/USDT). \emph{-} means that the corresponding method is either not implemented or unsuitable for corresponding setting. 
    % $\cdot / \cdot$ denotes the results of Alpha158 / Alpha360 on Qlib. 
    We retrieve the top 1000 signals with the highest probability for each experiment. The best performance is highlighted in \textbf{bold}. The second best is highlighted with \underline{underline}.
    }
    \scalebox{1.00}{
    \setlength{\tabcolsep}{7.0pt}
    \begin{tabular}{cl|ccc | ccc | cc}
    \toprule
        \multicolumn{2}{c|}{\multirow{2}*{Methods}} & \multicolumn{3}{c}{China's A-share stocks} & \multicolumn{3}{c}{Cryptocurrency} & \multicolumn{2}{c}{Ranking Count}\\ 
        \cmidrule(lr){3-5} \cmidrule(lr){6-8} \cmidrule(lr){9-10} 
        & & PR(\%) & WLR & AR & PR(\%) & WLR & AR & $1^{st}$ & $2^{nd}$\\
    \midrule
        \multirow{15}*{\begin{tabular}{c}Quantitative\\Investment\\Methods\end{tabular}}
        & \multicolumn{1}{l|}{OLS} & 45.5 & 1.209 & 4.33E-3 & 48.1 & 0.927 & 3.4E-5 & 0 & 0\\
        & \multicolumn{1}{l|}{MLP}    & 49.9 & 1.193 & 3.02E-3 & - & - & - & 0 & 0 \\
        & \multicolumn{1}{l|}{GRU}    & 51.3 & 1.114 & 3.02E-3 & 44.4 & 1.013 & 3.7E-5 & 0 & 0 \\  
        & \multicolumn{1}{l|}{LSTM}   & 55.0 & 1.106 & 5.53E-3 & 43.8 & 1.053 & 1.9E-5 & 0 & 0 \\
        & \multicolumn{1}{l|}{ALSTM}  & 51.9 & 1.133 & 3.24E-3 & 47.9 & 0.933 & 5.9E-5 & 0 & 0 \\
        & \multicolumn{1}{l|}{TabNet} & 51.8 & 1.299 & 5.14E-3 & 51.0 & 0.890 & 1.4E-5 & 0 & 0 \\
        & \multicolumn{1}{l|}{Transformer} & 53.2 & 1.230 & 5.73E-3 & 38.7 & 0.888 & -5.0E-5\hspace{0.3em} & 0 & 0 \\
        & \multicolumn{1}{l|}{Adamct} & 52.7 & \underline{1.309} & 5.73E-3 & 49.3 & \underline{1.177} & 1.3E-4 & 0 & \textbf{2} \\
        & \multicolumn{1}{l|}{LightGBM} & 55.0 & \textbf{1.331} & \underline{7.26E-3} & 51.0 & 0.890 & 1.4E-5 & \underline{1} & \underline{1} \\ 
        & \multicolumn{1}{l|}{XGBoost}  & 53.3 & 1.138 & 5.22E-3 & 53.3 & 0.678 & -3.0E-5\hspace{0.3em} & 0 & 0 \\ 
        & \multicolumn{1}{l|}{GATs}   & 52.7 & 1.237 & 6.26E-3 & - & - & - & 0 & 0 \\
        & \multicolumn{1}{l|}{SFM}    & 54.3 & 1.110 & 5.63E-3 & - & - & - & 0 & 0 \\
        & \multicolumn{1}{l|}{TFT}    & 50.7 & 1.184 & 3.92E-3 & - & - & - & 0 & 0 \\
        & \multicolumn{1}{l|}{DoubleEnsemble} & 54.0 & 1.225 & 5.75E-3 & - & - & - & 0 & 0\\
        & \multicolumn{1}{l|}{TCTS}           & 55.6 & 0.913 & 2.09E-3 & - & - & - & 0 & 0\\
        
    \midrule
        \multirow{3}*{\begin{tabular}{c}Time-series \\ Methods\end{tabular}}
        % & \multicolumn{1}{l|}{DLinear} & - & 52.1 & - & - & 1.120 & - & - & 3.88E-3 & - \\ 
        & \multicolumn{1}{l|}{iTransformer} & 53.8 & 1.095 & 4.01E-3 & - & - & - & 0 & 0\\
        & \multicolumn{1}{l|}{PatchTST}     & 53.0 & 1.274 & 5.17E-3 & - & - & - & 0 & 0\\
        & \multicolumn{1}{l|}{TimesNet}     & 55.5 & 1.131 & 6.16E-3 & - & - & - & 0 & 0\\
    \midrule
        \multirow{3}*{\begin{tabular}{c}Noisy Labels \\ Methods\end{tabular}}
        & \multicolumn{1}{l|}{CNLCU} & 52.6 & 1.233 & 5.03E-3 & 52.9 & \textbf{1.220}    & 1.2E-4 & \underline{1} & 0 \\ 
        & \multicolumn{1}{l|}{FINE}  & 55.3 & 1.070 & 4.35E-3 & \underline{56.3} & 0.863 & 9.7E-5 & 0 & \underline{1}\\ 
        & \multicolumn{1}{l|}{SEAL}  & \underline{56.6} & 1.200 & 5.95E-3 & 53.0 & 0.969 & 7.2E-5 & 0 & \underline{1} \\ 
    \midrule
        \multirow{3}*{Ours}
        & LA-Attention & \underline{56.6} & 1.142 & 5.27E-3 & 51.2 & 0.826 & 9.5E-5 & 0 & \underline{1}\\
        & RA-Labeling  & 55.2 & 1.038 & 3.53E-3 & 56.2 & 1.034 & \underline{1.4E-4} & 0 & \underline{1}\\
        & LARA         & \textbf{59.1} & 1.274 & \textbf{7.79E-3} & \textbf{57.8} & 1.059 & \textbf{1.5E-4} & \textbf{4} & 0\\
    \bottomrule
    \end{tabular}
    }
    \label{tab:appendix-whole-results}
    \vspace{-0.3cm}
\end{table*}

\section{Compared Methods}
\subsection{List of Competitors}
The main descriptions of all baselines are listed below:

\begin{itemize}[leftmargin=10pt]
\item\textbf{Ordinary Least Squares (OLS)} fits a linear model to minimize the residual square sum among observed targets. 

\item\textbf{Autoregressive Integrated Moving Average (ARIMA)} is a class of models that ``explains'' a given time series based on its own lags and the lagged forecast errors.
   
\item\textbf{Ridge} regression minimizes a penalized residual sum of squares by imposing a penalty on the size of the coefficients.

\item\textbf{Decision Trees} 
create a model that predicts target values by learning simple decision rules inferred from features.

\item\textbf{Bagging Regressor} is an ensemble estimator that fits base regressors on random subsets of original datasets and then aggregates individual predictions to form a final prediction. 

\item\textbf{AdaBoost~\cite{freund1997decision}} fits a sequence of weak learners on repeatedly modified sample weight of the data and then combines through a weighted majority vote to produce the final prediction.

\item\textbf{Multi-Layer Perceptron (MLP)} trains iteratively \emph{w.r.t} the loss function to update the parameters. This model optimizes the squared loss using the stochastic gradient descent. 

\footnotetext[2]{Short selling is not allowed in China’s A-share market without considering margin trading and also in the cryptocurrency market.}

\item\textbf{LightGBM} \cite{ke2017lightgbm} is an efficient implementation of gradient boosting decision tree (GBDT). This method also serves as the base classifier in our LARA framework.

\item \textbf{XGBoost~\cite{chen2016xgboost} and LightGBM~\cite{ke2017lightgbm}} are non-linear models based on gradient boosting trees.

\item \textbf{Transformer~\cite{vaswani2017attention}} utilizes the attention mechanism to explicitly model the relationship among different parts of input data.

\item \textbf{Adamct~\cite{jiang2022adamct}} proposes to adopt a global attention mechanism with a local convolutional filter to model both local and global dependencies of input data.

\item \textbf{LSTM~\cite{hochreiter1997long}} is the vanilla LSTM model, which obtains a sequential embedding; and then an FC layer is used to make the final prediction of return.

\item \textbf{GRU~\cite{chung2014empirical}} is an extended version of LSTM, which has a forget gating mechanism to control the information flow.

\item \textbf{ALSTM~\cite{qin2017dual}} adds an external attention layer into the vanilla model to adaptively aggregate hidden states' information of previous timestamps.

\item \textbf{GATs~\cite{velivckovic2017graph}} utilizes the Graph Neural Networks~(GNNs) to model the relationship between different stocks, and the attention scheme is incorporated into GNNs.

\item \textbf{SFM~\cite{zhang2017stock}} redesigns the recurrent neural networks by decomposing hidden states into multiple frequency components to model multi-frequency trading patterns.

\item \textbf{TFT~\cite{lim2019enhancing}} introduces Deep Momentum Networks to simultaneously learn both trend estimation and position sizing in a data-driven manner.

\item \textbf{TabNet~\cite{arik2020tabnet}} is a deep tabular data learning architecture, which uses sequential attention to choose which features to reason from at each decision step.

\item \textbf{DoubleEnsemble~\cite{zhang2020doubleensemble}} proposes an ensemble framework leveraging learning trajectory based sample reweighting and shufﬂing based feature selection.

\item \textbf{TCTS~\cite{wu2021temp}} introduces a learnable scheduler and adaptively selects auxiliary tasks with the main task.

\item \textbf{iTransformer~\cite{liu2023itransformer}} invert the time-series data to explore the correlated properties between different attributes using the transformer architectures.

\item \textbf{PatchTST~\cite{nie2022time}} divides the time-series data into patches to process the temporal features and makes the cross-sectional features independent to avoid overfitting.

\item \textbf{TimesNet~\cite{wu2022timesnet}} decomposes the time-series data into 2D space according to different time periods and process them using 2D convolution.

\item \textbf{CNLCU~\cite{xia2021sample}} dynamically selects training samples by analysing the prediction values between two models.

\item \textbf{FINE~\cite{kim2021fine}} removes the noisy data with the largest differences by analyzing the eigenvectors of data in each category.

\item \textbf{SEAL~\cite{chen2021beyond}} proposes an Self-Evolution Average Label to help the model remove the interference of noisy labels.

\end{itemize}

\subsection{Description of Noisy Labels Methods}
Learning with noisy labels is a common challenge in many real-world applications~\cite{bloomfield2009noise}. When dealing with such noisy labels, there are generally several approaches. One method involves evaluating the probability of different categories being misclassified as others, thereby establishing a soft-label~\cite{song2022learning}. However, this approach requires assuming the type of noise and may not be applicable to all datasets. Another method focuses on identifying noisy samples, modifying their labels, or removing these noisy samples~\cite{chen2021beyond,kim2021fine,xia2021sample}. These methods use different criteria to identify noisy samples or correct labels. However, they are suitable for datasets with a small amount of noise, but their performance on datasets with significant noise remains to be studied. The most crucial issue here is how to determine whether the modifications made to the dataset are genuinely corrective or if they are introducing additional noise

Price movement forecasting is notoriously difficult largely due to the financial market's inherently stochastic, dynamic, and volatile nature. Unlike noisy labels in the field of image classification~(such as tagging a cat as a dog), the fluctuation of financial market prices is heavily influenced by noise, making it difficult to visually determine whether the label is true for this type of data. Only a small fraction of the time is driven by genuinely informative data that leads to price changes. Due to this issue, simple label modifications or noisy sample removal can inadvertently increase uncertainty or eliminate the potentially profitable opportunities. From this perspective, when dealing with datasets containing significant noise, it is essential to focus precisely on the most promising samples~(selected by our LA-Attention) and apply targeted denoising techniques~(our RA-Labeling) to these specific samples. This approach is the most rational and suitable for such scenarios. Indeed, other methods for handling noisy labels may involve getting caught in a cycle of modifying labels within the noisy data, especially if the data itself is noisy and the labels are not particularly crucial.

\begin{table*}[htbp]
    \centering
    \caption{Quantitative comparisons among different methods on 512480.SH.
    \vspace{-0.3cm}
    }
    \scalebox{0.92}{
    \setlength{\tabcolsep}{6pt}
    \begin{tabular}{cl|cccc}
    \toprule
        \multicolumn{2}{c|}{Methods} & Precision(\%) & Win-Loss Ratio & Average Return & \#Transactions \\ 
    \midrule
        \multirow{2}*{Time Series} 
        & \multicolumn{1}{l|}{OLS} & $52.22_{\pm0.21}$ & $2.430_{\pm0.017}$ & $1.27\text{E-3}_{\pm4\text{E-6}}$ & 1000 \\ 
        & \multicolumn{1}{l|}{ARIMA} & $12.57_{\pm2.77}$ & $0.919_{\pm0.073}$ & $-6.00\text{E-5}_{\pm1\text{E-4}}\hspace{0.55em}$ & 1000 \\
    \midrule
        \multirow{6}*{Machine Learning} 
        & \multicolumn{1}{l|}{Ridge} & $53.58_{\pm0.22}$ & $2.754_{\pm0.009}$ & $1.29\text{E-3}_{\pm1\text{E-5}}$ & 1000 \\ 
        & \multicolumn{1}{l|}{Decision Trees} & $34.48_{\pm1.44}$ & $1.487_{\pm0.111}$ & $6.70\text{E-3}_{\pm5\text{E-5}}$ & 1000 \\ 
        & \multicolumn{1}{l|}{Bagging Regressor} & $62.14_{\pm1.56}$ & $2.187_{\pm0.183}$ & $1.61\text{E-3}_{\pm4\text{E-5}}$ & 1000 \\ 
        & \multicolumn{1}{l|}{AdaBoost} & $51.32_{\pm3.23}$ & $1.935_{\pm0.055}$ & $1.15\text{E-3}_{\pm8\text{E-5}}$ & 1000 \\
        & \multicolumn{1}{l|}{MLP} & \hspace{0.35em}$43.53_{\pm17.89}$ & $1.838_{\pm0.293}$ & $9.30\text{E-4}_{\pm5\text{E-4}}$  & 1000\\ 
        & \multicolumn{1}{l|}{LightGBM} & $70.16_{\pm0.89}$ & $2.872_{\pm0.106}$ & $1.66\text{E-3}_{\pm2\text{E-5}}$ & 1000 \\
    \midrule
        \multirow{3}*{Ours}
         & LA-Attention & $78.36_{\pm1.14}$ & $\bm{2.934_{\pm0.241}}$ & $1.96\text{E-3}_{\pm4\text{E-5}}$ & 1000 \\
         & RA-Labeling & $71.03_{\pm0.60}$ & $2.913_{\pm0.097}$ & $1.68\text{E-3}_{\pm1\text{E-5}}$ & 1000 \\
         & LARA & $\bm{79.53_{\pm0.67}}$ & $2.933_{\pm0.221}$ & $\bm{1.98\text{E-3}_{\pm2\text{E-5}}}$ & 1000 \\
    \bottomrule
    \end{tabular}
    }
    \label{tab:exp-baseline-ablation-512480}
\end{table*}

\begin{table*}[htp]
    \centering
    \caption{Quantitative comparisons among different methods on 515050.SH ETF. 
    \vspace{-0.3cm}
    }
    \scalebox{0.92}{
    \begin{tabular}{cl|cccc}
    \toprule
        \multicolumn{2}{c|}{Methods} & Precision(\%) & Win-Loss Ratio & Average Return & \#Transactions \\
    \midrule
        \multirow{2}*{Time Series} 
        & \multicolumn{1}{l|}{OLS} & $55.23_{\pm0.10}$ & $1.369_{\pm0.001}$ & $1.37\text{E-3}_{\pm0\text{E-5}}$ & 1000 \\
        & \multicolumn{1}{l|}{ARIMA} & $9.45_{\pm0.00}$ & $1.006_{\pm0.000}$ & $-8.00\text{E-5}_{\pm0\text{E-5}}$ & 1000 \\
    \midrule
        \multirow{6}*{Machine Learning} 
        & \multicolumn{1}{l|}{Ridge} & $46.24_{\pm0.02}$ & $1.393_{\pm0.002}$ & $1.18\text{E-3}_{\pm0\text{E-5}}$ & 1000 \\
        & \multicolumn{1}{l|}{Decision Trees} & $20.60_{\pm2.20}$ & $1.204_{\pm0.030}$ & $4.20\text{E-4}_{\pm6\text{E-5}}$ & 1000 \\ 
        & \multicolumn{1}{l|}{Bagging Regressor} & $40.95_{\pm1.19}$ & $1.465_{\pm0.077}$ & $1.04\text{E-3}_{\pm1\text{E-5}}$ & 1000 \\
        & \multicolumn{1}{l|}{AdaBoost} & $38.38_{\pm2.26}$ & $1.400_{\pm0.077}$ & $9.80\text{E-4}_{\pm6\text{E-5}}$ & 1000 \\
        & \multicolumn{1}{l|}{MLP} & $14.62_{\pm4.37}$ & $1.131_{\pm0.077}$ & $2.90\text{E-4}_{\pm2\text{E-4}}$ & 1000 \\
        & \multicolumn{1}{l|}{LightGBM} & $41.21_{\pm1.04}$ & $1.364_{\pm0.079}$ & $1.15\text{E-3}_{\pm2\text{E-5}}$ & 1000 \\
    \midrule
        \multirow{3}*{Ours}
         & LA-Attention & $56.73_{\pm1.15}$ & $1.586_{\pm0.099}$ & $\bm{1.41\text{E-3}_{\pm3\text{E-5}}}$ & 1000 \\
         & RA-Labeling & $41.51_{\pm0.78}$ & $1.362_{\pm0.035}$ & $1.16\text{E-3}_{\pm1\text{E-5}}$ & 1000 \\
         & LARA & $\bm{56.89_{\pm0.76}}$ & $\bm{1.595_{\pm0.119}}$ & $\bm{1.41\text{E-3}_{\pm3\text{E-5}}}$ & 1000 \\
    \bottomrule
    \end{tabular}
    }
    
    \label{tab:exp-baseline-ablation-515050}
\end{table*}

\begin{table*}[htp]
    \centering
    \caption{Comparison experimental comparisons among different methods on 512880.SH ETF. 
    \vspace{-0.3cm}
    }
    \scalebox{0.92}{
    \begin{tabular}{cl|cccc}
    \toprule
        \multicolumn{2}{c|}{Methods} & Precision(\%) & Win-Loss Ratio & Average Return & \#Transactions \\ 
    \midrule
        \multirow{2}*{Time Series} 
        & \multicolumn{1}{l|}{OLS}   & $51.95_{\pm0.15}$ & $1.055_{\pm0.004}$ & 9.80\text{E-4}_{\pm1\text{E-5}} & 1000 \\
        & \multicolumn{1}{l|}{ARIMA} & $21.04_{\pm0.16}$ & $1.024_{\pm0.002}$ & 6.00\text{E-5}_{\pm0\text{E-5}} & 1000 \\
    \midrule
        \multirow{6}*{Machine Learning} 
        & \multicolumn{1}{l|}{Ridge} & $58.21_{\pm0.20}$ & $1.172_{\pm0.006}$               & $\bm{1.30\text{E-3}_{\pm1\text{E-5}}}$ & 1000 \\
        & \multicolumn{1}{l|}{Decision Trees} & $34.47_{\pm3.38}$ & $1.021_{\pm0.088}$      & $4.60\text{E-4}_{\pm1\text{E-4}}$ & 1000 \\
        & \multicolumn{1}{l|}{Bagging Regressor} & $43.20_{\pm1.66}$ &$ 1.142_{\pm0.061}$   & $1.03\text{E-3}_{\pm1\text{E-4}}$ & 1000 \\
        & \multicolumn{1}{l|}{AdaBoost} & $50.12_{\pm4.00}$ & $\bm{1.241_{\pm0.107}}$       & $1.19\text{E-3}_{\pm2\text{E-4}}$ & 1000 \\
        & \multicolumn{1}{l|}{MLP} & $32.24_{\pm5.70}$ & $1.000_{\pm0.108}$                 & $1.90\text{E-4}_{\pm4\text{E-4}}$ & 1000 \\
        & \multicolumn{1}{l|}{LightGBM} & $70.36_{\pm0.67} $& $1.049_{\pm0.062}$            & $8.70\text{E-4}_{\pm1\text{E-5}}$ & 1000 \\
    \midrule
        \multirow{3}*{Ours}
         & LA-Attention & $70.88_{\pm2.18}$ & $1.132_{\pm0.104}$ & $1.22\text{E-3}_{\pm6\text{E-5}}$ & 1000 \\
         & RA-Labeling  & $70.57_{\pm0.23}$ & $0.993_{\pm0.053}$ & $8.60\text{E-4}_{\pm1\text{E-5}}$ & 1000 \\
         & LARA         & $\bm{74.60_{\pm0.81}}$ & $1.034_{\pm0.171}$ & $1.12\text{E-3}_{\pm3\text{E-5}}$ & 1000 \\
    \bottomrule
    \end{tabular}
    }
    \label{tab:exp-baseline-ablation-512880}
\end{table*}

\begin{table*}[htp]
    \centering
    \caption{Comparison experimental comparisons among different methods on 159915.SZ ETF. 
    \vspace{-0.3cm}
    }
    \scalebox{0.92}{
    \begin{tabular}{cl|cccc}
    \toprule
        \multicolumn{2}{c|}{Methods} & Precision(\%) & Win-Loss Ratio & Average Return & \#Transactions \\ 
    \midrule
        \multirow{2}*{Time Series} 
        & \multicolumn{1}{l|}{OLS}   & $44.67_{\pm0.09}$ & $\bm{2.251_{\pm0.048}}$ & $\bm{1.11\text{E-3}_{\pm0\text{E-5}}}$ & 1000 \\
        & \multicolumn{1}{l|}{ARIMA} & $4.89_{\pm0.08}$  & $0.943_{\pm0.005}$      & $-1.50\text{E-4}_{\pm1\text{E-5}}$ & 1000 \\
    \midrule
        \multirow{6}*{Machine Learning} 
        & \multicolumn{1}{l|}{Ridge} & $36.68_{\pm0.08}$ & $2.114_{\pm0.012}$               & $9.60\text{E-4}_{\pm 0\text{E-5}}$ & 1000 \\
        & \multicolumn{1}{l|}{Decision Trees} & $16.42_{\pm2.75}$ & $1.329_{\pm0.102}$      & $3.90\text{E-4}_{\pm 7\text{E-5}}$ & 1000 \\
        & \multicolumn{1}{l|}{Bagging Regressor} & $31.00_{\pm2.22}$ & $1.787_{\pm0.127}$   & $7.80\text{E-4}_{\pm 4\text{E-5}}$ & 1000 \\
        & \multicolumn{1}{l|}{AdaBoost} & $32.22_{\pm2.02}$ & $1.735_{\pm0.138}$            & $8.20\text{E-4}_{\pm 4\text{E-5}}$ & 1000 \\
        & \multicolumn{1}{l|}{MLP} & $9.38_{\pm5.83}$ & $1.118_{\pm0.237}$                  & $1.10\text{E-4}_{\pm 2\text{E-5}}$ & 1000 \\
        & \multicolumn{1}{l|}{LightGBM} & $36.25_{\pm0.92}$ & $2.013_{\pm0.142}$            & $9.70\text{E-4}_{\pm 2\text{E-5}}$ & 1000 \\
    \midrule
        \multirow{3}*{Ours}
         & LA-Attention  & $44.11_{\pm0.98}$ & $1.879_{\pm0.132}$      & $1.06\text{E-3}_{\pm 2\text{E-5}}$ & 1000 \\
         & RA-Labeling   & $35.92_{\pm0.32}$ & $1.953_{\pm0.155}$      & $9.80\text{E-4}_{\pm 1\text{E-5}}$ & 1000 \\
         & LARA          & $\bm{45.47_{\pm1.30}}$ & $1.834_{\pm0.191}$ & $1.08\text{E-3}_{\pm 2\text{E-5}}$ & 1000 \\
    \bottomrule
    \end{tabular}
    }
    \label{tab:exp-baseline-ablation-159915}
\end{table*}

\begin{figure*}[htbp]
	\centering
	\includegraphics[width=1.\textwidth]{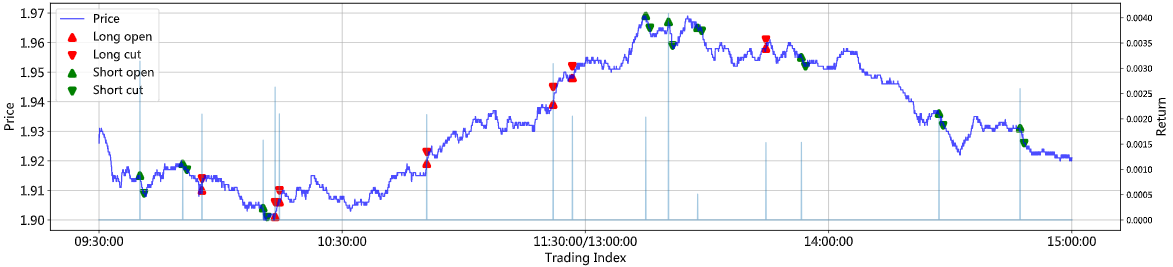}
	\caption{Overview of open-close positions on 512480.SH.}
	\label{fig:open-cut-512480}
\end{figure*}

\begin{figure*}[htbp]
	\centering
	\includegraphics[width=1.\textwidth]{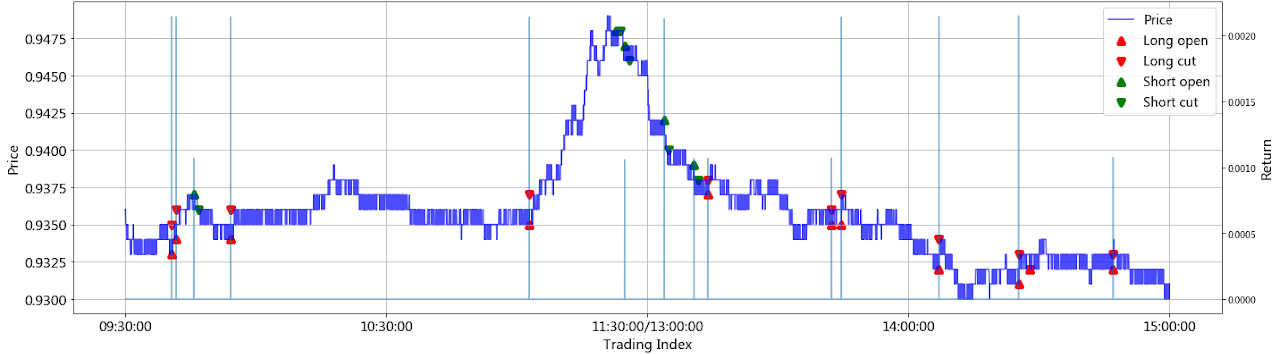}
	\caption{Overview of open-close positions on 512880.SH.}
	\label{fig:open-cut-512880}
\end{figure*}

\begin{figure*}[htbp]
	\centering
	\includegraphics[width=1.\textwidth]{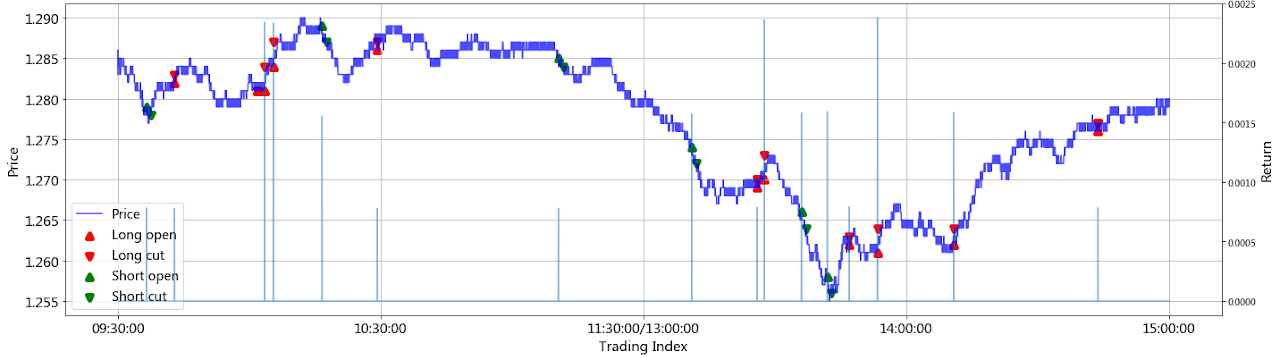}
	\caption{Overview of open-close positions on 515050.SH.}
	\label{fig:open-cut-515050}
\end{figure*}

\begin{figure*}[htbp]
	\centering
	\includegraphics[width=1.\textwidth]{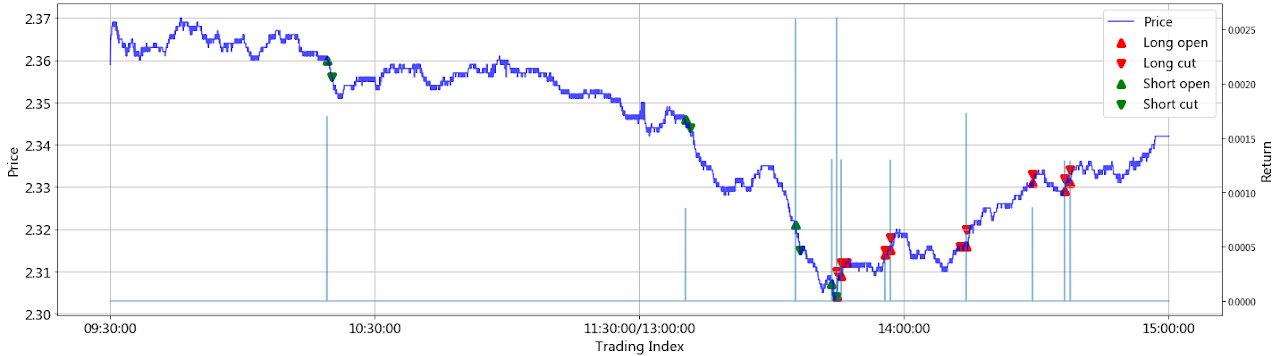}
	\caption{Overview of open-close positions on 159915.SZ.}
	\label{fig:open-cut-159915}
\end{figure*}

\begin{figure*}[htbp]
    \centering
    \includegraphics[width=.83\textwidth]{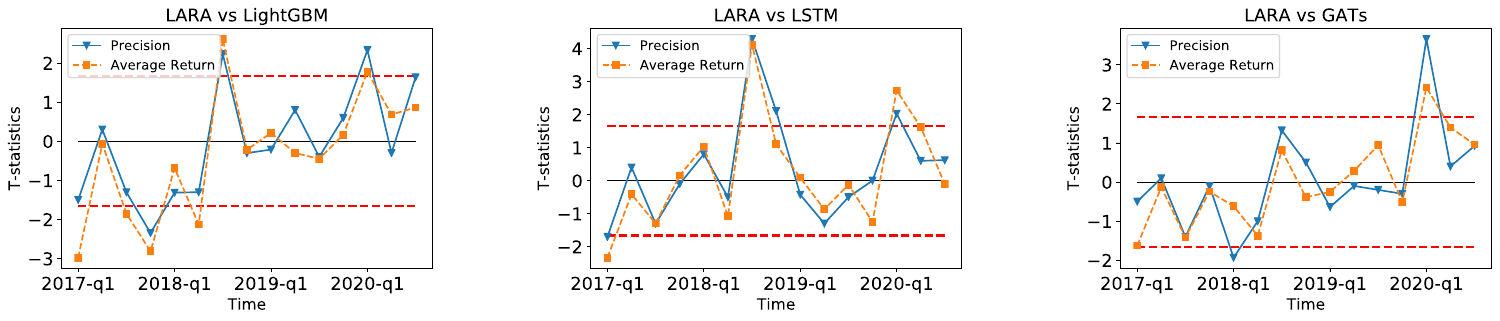}
	\caption{Statistical tests of Precision and Average Return on China's A-share market quarterly. If the curve is above the dotted red line (black line), our proposed framework LARA is significantly better (slightly better) than the corresponding method, and vice versa~(significance level $\alpha$ equals to 0.05).}
	\label{fig:statistical-test}
\end{figure*}

\section{More Experimental Results}
\subsection{Performance Comparison on Stocks and Crypto}
We have conducted extensive experiments and comparative analysis for our proposed LARA.
Due to the space limitation, only a part of representative results is presented in the main text. The complete results of all experiments for stocks and crypto are shown in Table~\ref{tab:appendix-whole-results}. It can be find that LARA significantly outperforms other methods on the prediction precision and the average return metrics.

\subsection{Parameter Study}
\begin{figure}[tp]
	\includegraphics[width=.49\textwidth]{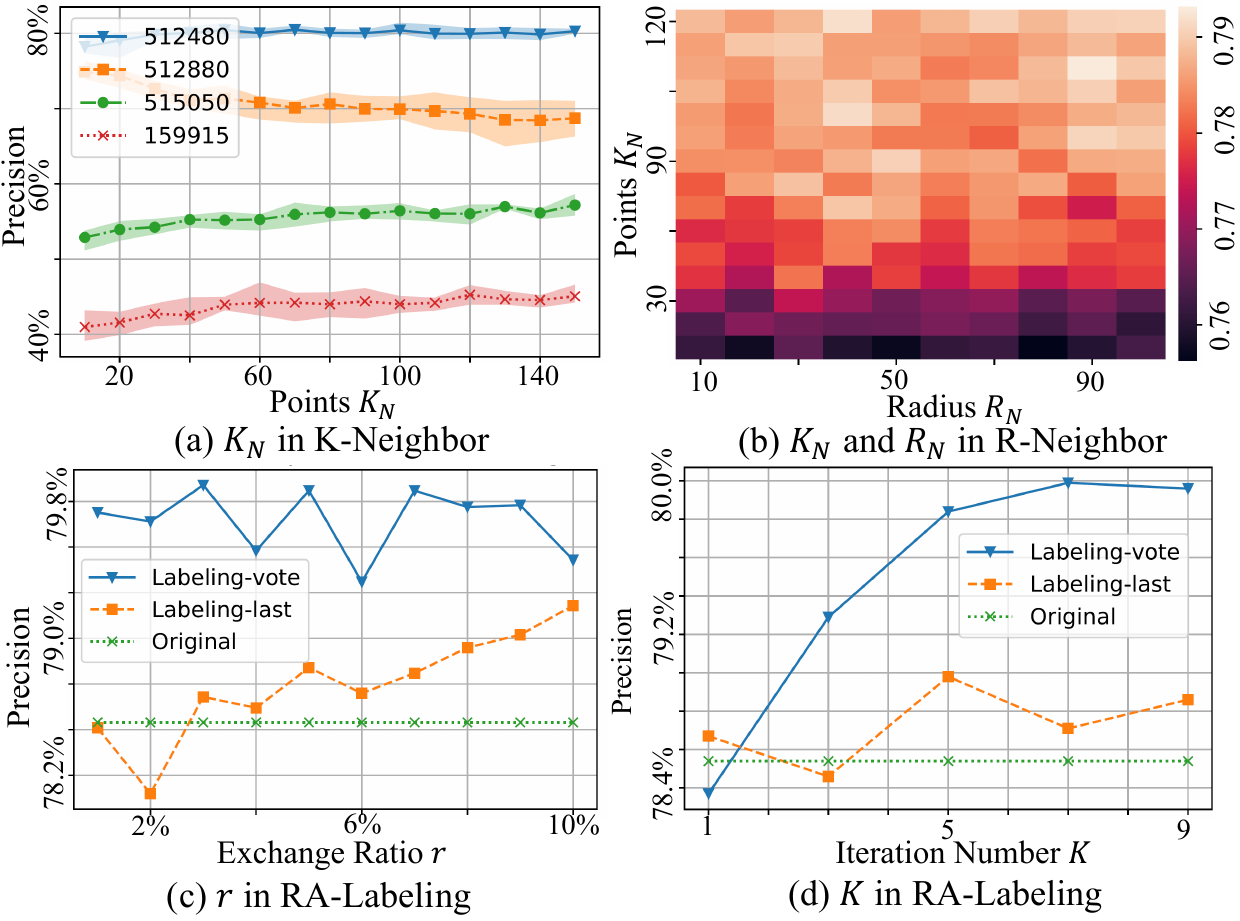}
	\caption{Hyperparameter study. (a)(b) $K_N$ and $R_N$ in K-Neighbor and R-Neighbor. (c)(d) $r$ and $K$ in RA-Labeling. Results of the experiments in (b)(c)(d) are obtained on 512480.}
	\label{fig:parameter-study}
\end{figure}

\paragraph{Hyperparameter Study of LA-Attention.} 
We propose two schemes to define the neighbors in LA-Attention: K-Neighbor and R-Neighbor (Sec.~\ref{sec:attention}).
We investigate the sensitivity of the corresponding hyperparameters: $K_N$ in K-Neighbor and $K_N$, $R_N$ in R-Neighbor.
As shown in Fig.~\ref{fig:parameter-study}(a), when $K_N$ in K-Neighbor varies from $20$ to $140$, the precision of most ETFs gradually increases.
The same situation occurs in Fig. \ref{fig:parameter-study}(b). The larger number of neighbors R-Neighbor attends to, the better performance we can obtain. However, it costs more time when attending to more neighbors, which is a trade-off between time and performance. 
Besides, when we vary radius $R_N$ from $10$ to $100$ using a fixed $K_N$, R-Neighbor achieves relatively stable performance.
These results suggest that LA-Attention does not rely on the heavy tuning of hyperparameters to achieve a satisfactory performance.

\paragraph{Hyperparameter Study of RA-Labeling.}
We conduct experiments to analyze the robustness of two combination schemes in RA-Labeling (Sec.~\ref{sec:bi-level}) with different iteration numbers $K$ and exchange ratios $r$. 
In Fig.~\ref{fig:parameter-study}(c)(d), it is evident that \emph{labeling-last}~($C_{\text{Last}}$) achieves superior performance as $r$ and $K$ increase. 
Furthermore, \emph{labeling-vote}~($C_{\text{Vote}}$) largely enhances precision compared to \emph{labeling-last}, indicating that combining all the learned predictors is a good choice in RA-Labeling. 
The performance of \emph{Labeling-vote} reaches saturation when $r$ is exceeds $2\%$ and $K$ surpasses 7.

\subsection{Performance Comparison on ETFs.}

We present quantitative comparisons among different methods on four ETFs, including 159915.SZ, 512480.SH, 512880.SH, 515050.SH. 
For a comprehensive comparison, we use widely-used methods from three representative categories: traditional time series analysis models, machine learning based models, and LARA variants. The \cref{tab:exp-baseline-ablation-512480,tab:exp-baseline-ablation-515050,tab:exp-baseline-ablation-512880,tab:exp-baseline-ablation-159915} illustrate the comparative results between LARA and other methods.
In Table~\ref{tab:exp-baseline-ablation-512480}, we find that LARA consistently outperforms other methods by a large margin~(\emph{e.g.}, 9.37\% improvements in precision compared with LightGBM), which validates the effectiveness of our proposed framework. 
In \cref{tab:exp-baseline-ablation-515050,tab:exp-baseline-ablation-512880,tab:exp-baseline-ablation-159915}, LARA consistently achieves the best performance in precision, which indicates that LARA can accurately capture the trading opportunities.

\subsection{Trading Transactions}

We plot the open-close positions in \cref{fig:open-cut-512480,fig:open-cut-512880,fig:open-cut-515050,fig:open-cut-159915} to illustratively explain how our proposed LARA framework works. LARA achieves favorable profit in both long and short positions. Even though the forecasting target is 0.1\%, more than half of the transactions earn more than 0.2\%, and some even reach 0.4\%, which shows that LARA has indeed captured satisfactory and profitable trading opportunities.
Besides, we can find that during the up-trend period, we open long positions (red triangles in Fig. \ref{fig:open-cut-512480}); in the down-trend period, we open short positions (blue triangles in Fig. \ref{fig:open-cut-512480}). 
Obviously, it is a rational way to open positions when there is a stronger tendency and do nothing when the price fluctuates around value.

As shown in Fig.~\ref{fig:statistical-test}, we compare with three machine learning models, \emph{i.e.,} LightGBM, LSTM, and GATs.
For each method, we select the top 200 signals with the highest predicted probability value in each quarter~(1800 signals in total) and perform the t-statistical test of Precision and Average Return between LARA and the corresponding method quarterly~(significance level $\alpha$ equals 0.05). If the curve is above the dotted red line, it represents that LARA is signiﬁcantly better than the corresponding model, and vice versa. We can empirically find that from 2019-q1 to 2020-q2, LARA achieves significant performance compared with other machine learning based models. From 2017-q1 to 2019-q1, LARA is on par with other baseline models. 
We postulate that the reason could be attributed to the violent fluctuation of assets price during this period~\cite{de2018advances}.

\subsection{Framework Evaluation}
LARA is a generic framework for price movement forecasting. In the main text of the paper, we utilize the LightGBM as the predictor and have achieved great performance. As shown in Table~\ref{tab:appendix-framework-evaluation}, we change the predictor from OLS, MLP and DoubleEnsemble~\cite{zhang2020doubleensemble} to verify whether this framework is effective for different models. It shows that LARA, as a framework, can consistently enhance the predictive precision of the base predictors and and improve the average return. This indicates that LARA is an effective generic framework for price movement forecasting.

In the actual quantitative investment scenarios, data is usually presented in tabular form as factors. The metric learning module can handle this type of data well, but it is unable to process raw time-series data. Therefore, when choosing the base predictor here, we select the base predictors~(OLS, MLP and DoubleEnsemble) especially for tabular data. Further research is needed for other time-series models.

\begin{table}[htbp]
    \centering
    \caption{Ablation studies with LARA using different base predictors. The best performance is highlighted in \textbf{bold}.}
    \scalebox{1.00}{
    \setlength{\tabcolsep}{7.5pt}
    \begin{tabular}{c|ccc}
    \toprule
        \multirow{2}*{Methods} & \multicolumn{3}{c}{China's A-share stocks} \\
        \cmidrule(lr){2-4}
         & PR~(\%) & WLR & AR  \\
    \midrule
        OLS     & 45.5 & \textbf{1.209} & 4.33E-3 \\ 
        + LARA  & \textbf{54.0} & 1.166 & \textbf{5.01E-3}\\
    \midrule
        MLP     & 49.9 & 1.193 & 3.02E-3 \\
        + LARA  & \textbf{51.8} & \textbf{1.393} & \textbf{4.29E-3}  \\
    \midrule 
        DoubleEnsemble & 54.0 & 1.225 & 5.75E-3 \\
        + LARA         & \textbf{56.6} & \textbf{1.230} & \textbf{6.24E-3} \\
    \bottomrule
    \end{tabular}
    }
    \label{tab:appendix-framework-evaluation}
\end{table}

\subsection{Masked Attention Scheme}
\label{sec:appendix:example}
We run the \emph{masked attention scheme} on a simplified example for further study in Fig.~\ref{fig:nn-example}.
We can obtain \emph{samples with high $p_\vx$} in the blue region calculated by the \emph{masked attention scheme}, whose labels are indeed dominated by the positive ones. 
We optimize an SVM classifier with the Gaussian kernel on the whole data, leading to the blue decision boundary located in the mixing regions.
However, if we optimize the classifier only on the \emph{samples with high $p_\vx$}, we can get the red decision boundary located in the blue region, which is far from the middle mixing regions. Thus it can be more robust to the noise of datasets and generate more profitable signals.
\begin{figure}[htbp]
    \centering
    \includegraphics[width=7.5cm]{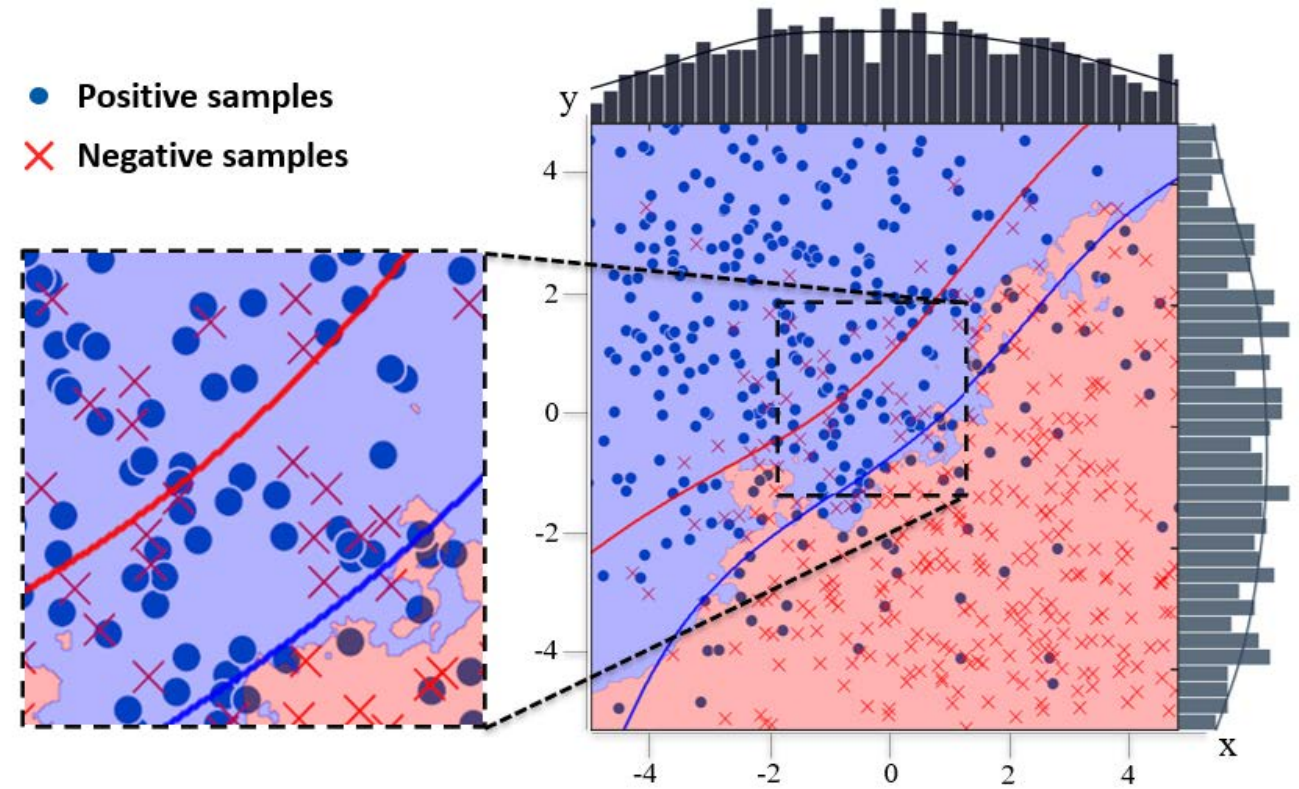}
    % \vspace{-0.4cm}
    \caption{A running example of the \emph{masked attention scheme}. Randomly sample 400 samples from $\mathcal{N}((-2,2), 8I_2)$ and $\mathcal{N}((2,-2), 8I_2)$ as positive and negative samples, respectively. The blue region denotes the \emph{samples with high $p_\vx$} calculated by the \emph{masked attention scheme}. The blue curve is the decision boundary of an SVM classifier with the Gaussian kernel training on the whole set, and the red curve is that training only on the \emph{samples with high $p_\vx$}. The left figure is the enlarged view of the area near the decision boundary.}
    \label{fig:nn-example}
    % \vspace{-0.4cm}
\end{figure}

\subsection{Ablation Study on Average Return}
Following the experimental settings in Fig.~\ref{fig:experiment-all} left, we perform experiments on LARA and the corresponding machine learning methods in terms of average return under different $\#$Transactions in Fig.~\ref{fig:trades-diff}. We find that LARA consistently outperforms OLS and LightGBM, which highlights the effectiveness of LARA across different trading frequencies.
\begin{figure}[htbp]
	\centering
	\includegraphics[width=.45\textwidth]{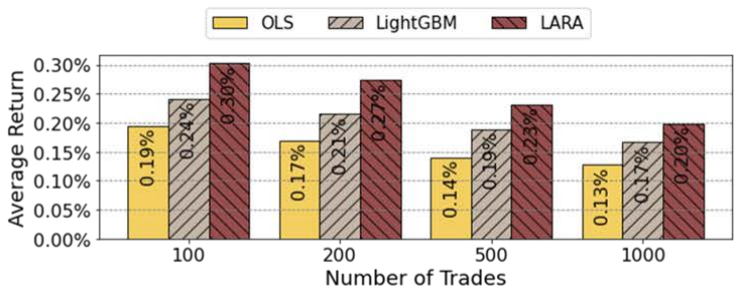}
	\caption{Comparisons with the different number of trades among three methods over Average Return on 512480.SH.}
	\label{fig:trades-diff}
\end{figure}

\section{More discussions on LARA}
\subsection{Intuition on LARA} 
We explain the motivation of our proposed framework with an intuitive analogy of evaluating students’ academic performance.
According to the history of students' performance, we regard the excellent students as positive samples and the ordinary students as negative samples, as shown in Fig.~\ref{fig_price}. 
Excellent students typically get higher scores than ordinary ones in a single exam, just like the potentially profitable samples in the context of financial datasets.
It inspires us to extract the potentially profitable samples~(excellent students) first
and then construct a more accurate classifier on these selected samples~(\ie, Fig.~\ref{fig_price}(a)-(b)).
If only one historical exam is observed, it is too hard for us to make a comprehensive evaluation so that we may miss some excellent students and choose the ordinary ones by mistake. 
Moreover, the ordinary students (red/blue \emph{noisy samples} located in Fig. \ref{fig_price}(a)/Fig. \ref{fig_price}(b)) mixed into the group of excellent students can be easily distinguished via multiple exams. 
Thus, it inspires us to further denoise the labels of \emph{noisy samples} with multiple iterative evaluations.

\begin{figure}[htbp]
	\centering
	\includegraphics[width=.49\textwidth]{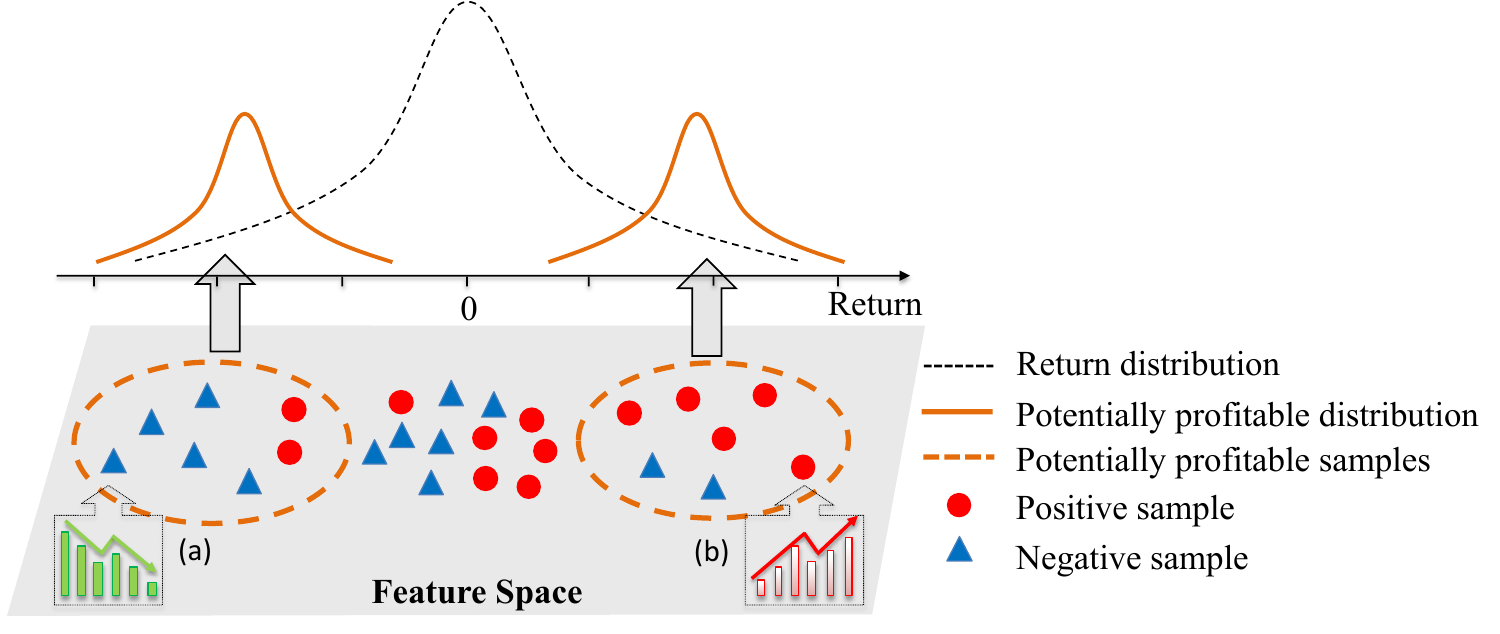}
	\caption{An example to illustrate our intuition. The half top figure represents the probability density function~(PDF) of return over corresponding samples~(best viewed in color).}
	\label{fig_price}
\end{figure}
\begin{figure}[htbp]
	\centering
	\includegraphics[width=.45\textwidth]{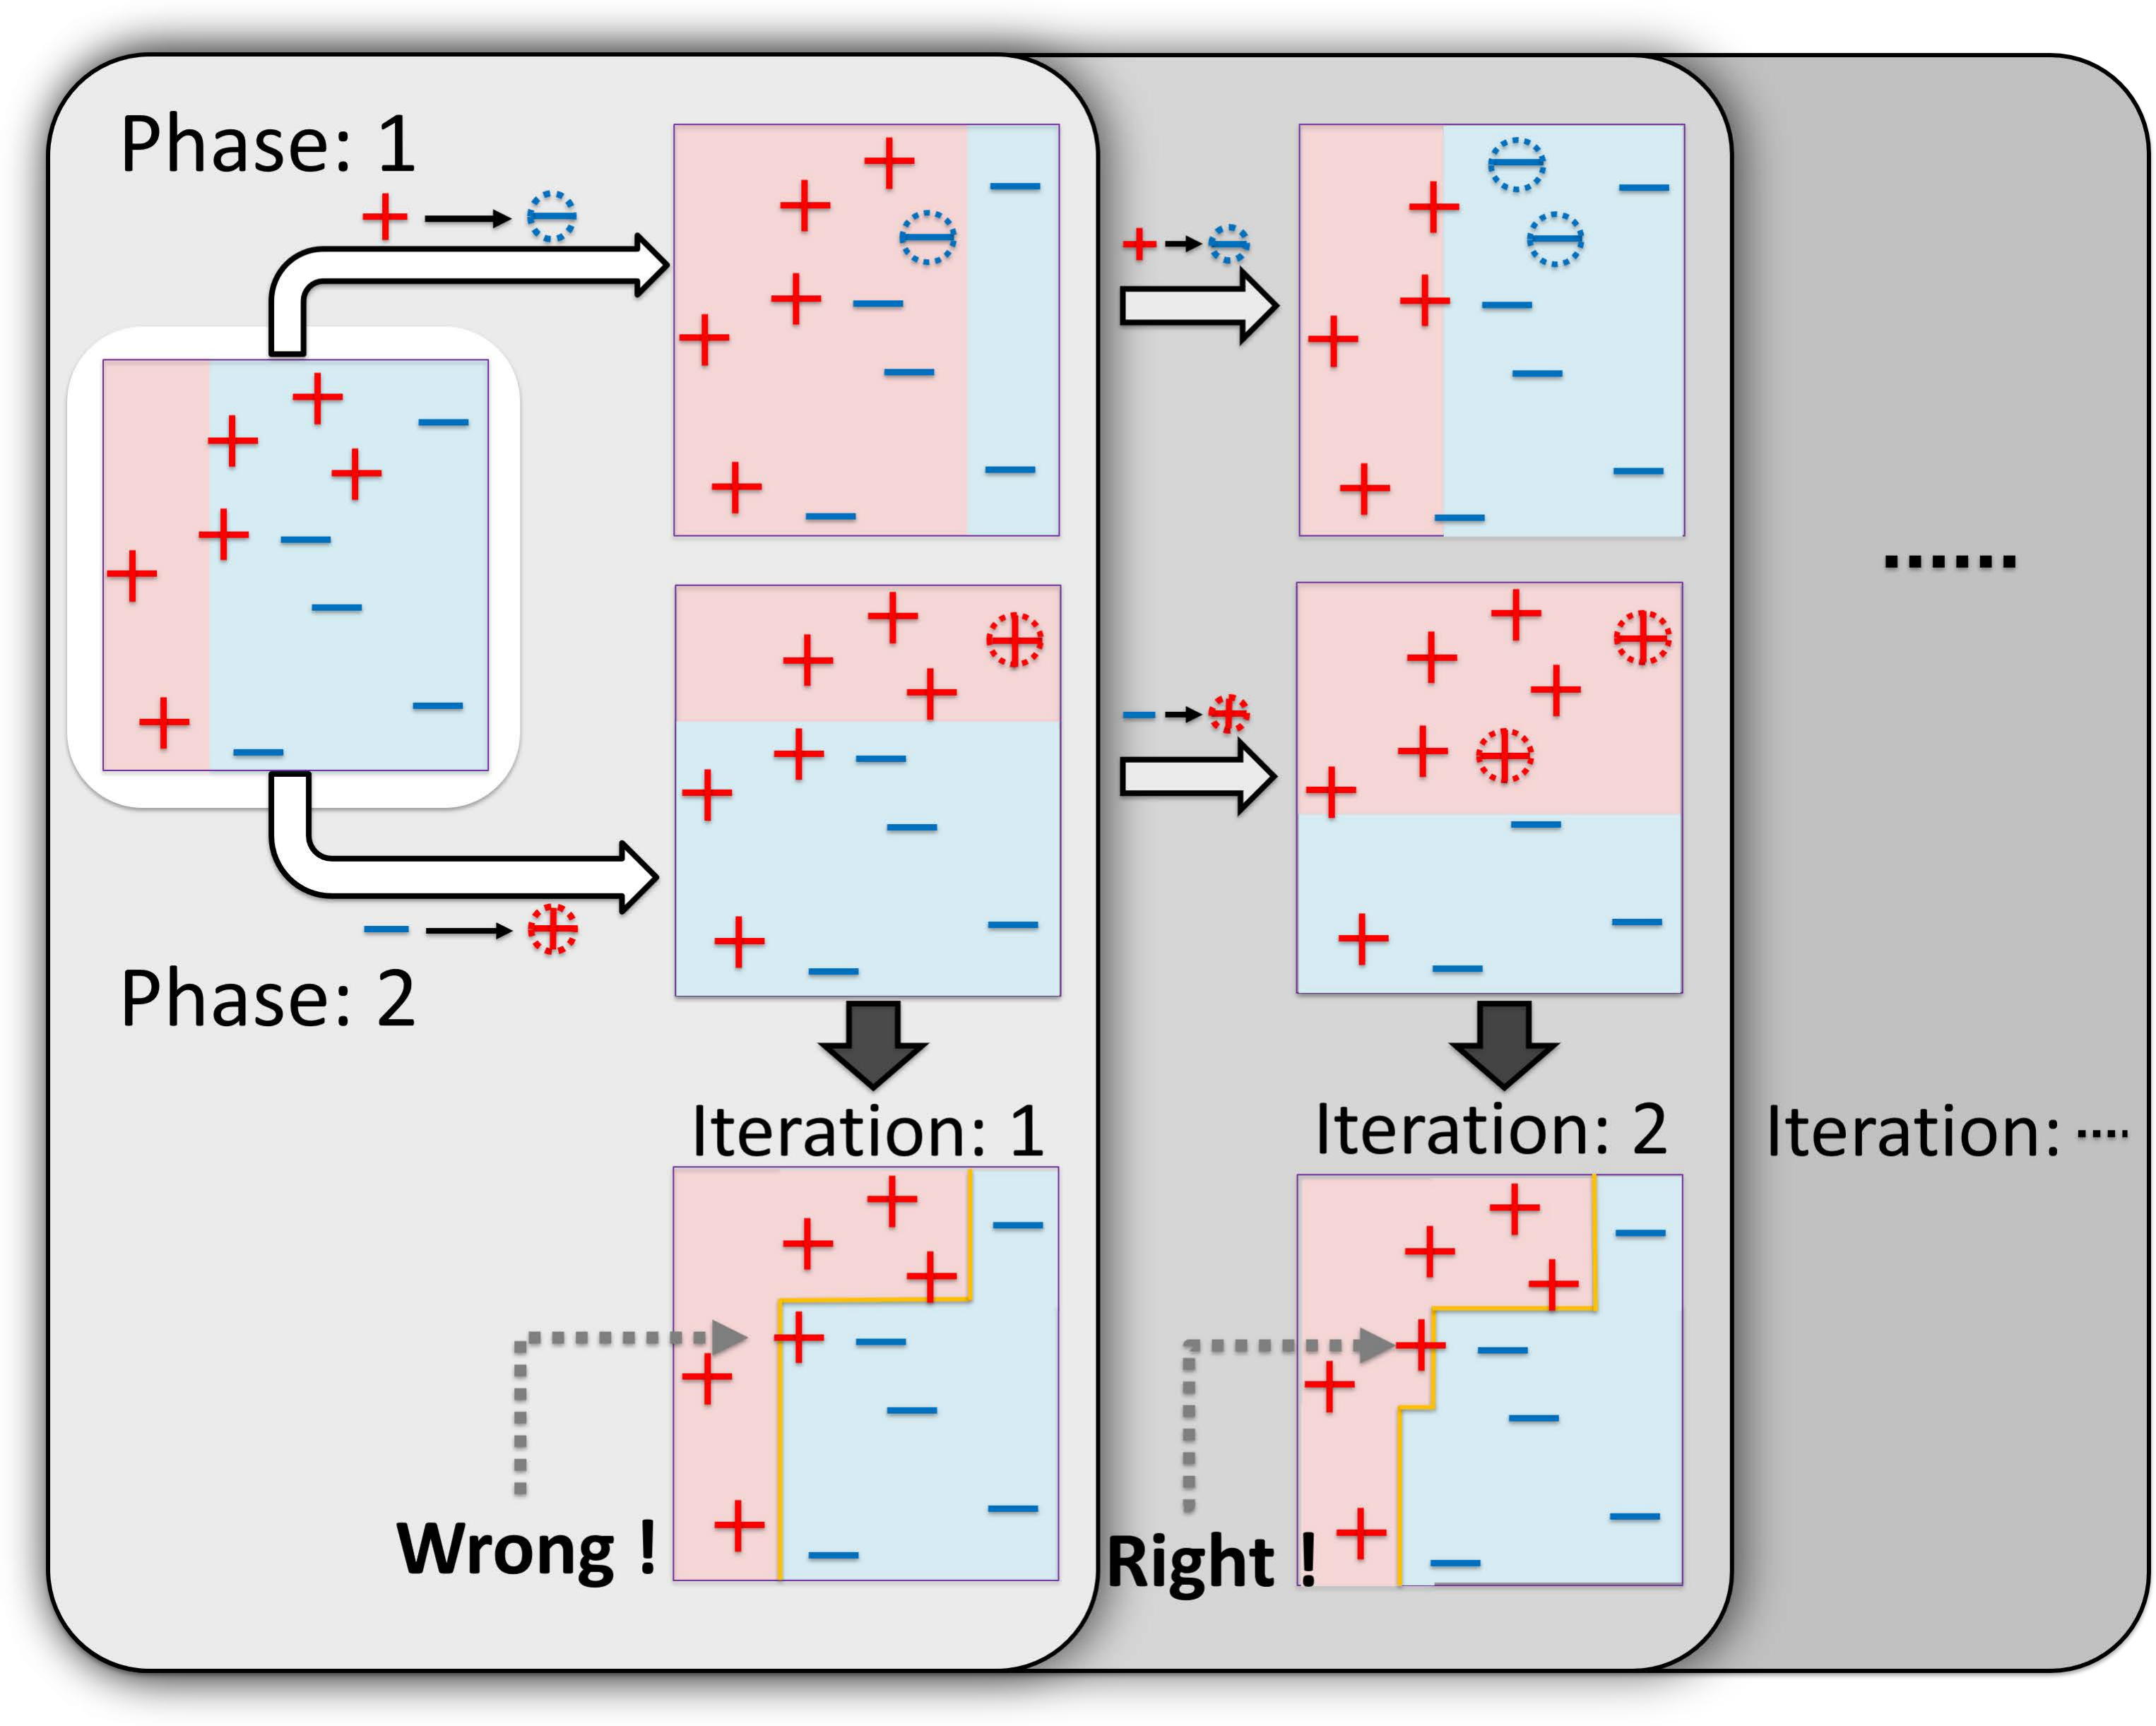}
% 	\vspace{-0.2cm}
	\caption{The illustration for the \emph{Iterative Refinement Labeling} method. The plus signs mean the positive samples and the minus signs mean the negative samples. The dotted circle means resetting the label of samples to the opposite one. The decision areas are represented in different colors~(Best viewed in color).
	}
	\label{fig_bi-level}
\end{figure}

\subsection{RA-Labeling}
We provide an illustrative example using the vote combining method, as shown in Fig.~\ref{fig_bi-level}. It shows that, at iteration $1$, the weak learners can discriminate the vast majority of samples correctly, except for only one misclassified sample. At iteration $2$, the algorithm further classifies all samples correctly after adaptively resetting the labels of two noisy samples and combining two more predictors. Finally, we combine all the trained models so far to boost the performance of predictors.

\subsection{Computational Complexity}
\label{appendix:complexity}
Due to the low feature dimension in our task (only 40), the optimization speed of $d \times d$ sparse Mahalanobis distance matrix in Metric learning (SDML) is fast. 
We denote $N$ and $N_{\text{test}}$ as the number of training data and testing data, respectively.
Let $d$ be the feature dimension.
For LA-Attention, the main time consumption is to search for neighbors of input samples, and we adopt the approximate nearest neighbor search method, \ie,~HNSW~\cite{malkov2018efficient}. 
HNSW costs $\mathcal{O}\left(N \log N \right)$ time for the construction of the data structure.
There are $(N+N_{\text{test}})$ samples needed to search for neighbors, and each of them takes $\mathcal{O}\left(\log N\right)$ time. 
Hence, it takes $\mathcal{O}\left(\left(2N+N_{\text{test}}\right)\log N\right)$ time in LA-Attention in total.
In addition, we define the time for constructing one estimator as $T_c$ in \emph{LightGBM} \cite{ke2017lightgbm}. Let $N_l$ be the number of estimators and $T_p$ be the time for predicting the testing data. RA-Labeling repeats the training and testing process for $K$ times, thus, the time cost is $\mathcal{O}\left(K\left(N_lT_c + T_p\right)\right)$ in total. Note that searching for neighbors in LA-Attention and predicting results via tree estimators can all be well paralleled, so we can react quickly in the actual financial market.

\section{Technical Factors}
In this section, we describe the technical factors we used in the ETFs and crypto. We used five-level limit order book data, and the specific atrtibute symbols are defined as shown in Table~\ref{tab:appendix-definition}.
\begin{table}[htbp]
    \centering
    \caption{Definition of the symbols.}
    \scalebox{1.00}{
    \setlength{\tabcolsep}{7.5pt}
    \begin{tabular}{c|l}
    \toprule
        Symbol & Meaning \\
    \midrule
        $av_i$ & $i$-th ask volume~($1 \leq i \leq 5$) \\ 
        $bv_i$ & $i$-th bid volume~($1 \leq i \leq 5$) \\ 
        $ap_i$ & $i$-th ask price~($1 \leq i \leq 5$) \\ 
        $bp_i$ & $i$-th bid price~($1 \leq i \leq 5$) \\ 
        $mid$  & $(ap_1 + bp_1) / 2$ \\
        shift(data, N) & Shift data index by N of periods \\
    \bottomrule
    \end{tabular}
    }
    \label{tab:appendix-definition}
\end{table}
Then，we define the factors as follows:
\paragraph{Volume Ratio} It reflects the supply and demand of investment behavior
\begin{equation}
    VOLR = \beta_1 \frac{bv_1 - av_1}{bv_1 + av_1} + \beta_2 \frac{bv_2 - av_2}{bv_2 + av_2} + \beta_3 \frac{bv_3 - av_3}{bv_3 + av_3}
\end{equation}
\paragraph{Price Percentage Change} It is a simple mathematical concept that represents the degree of change over time. It is used for many purposes in finance, often to represent the price change of a security.
\begin{equation}
    PCTN = \frac{mid-shift(mid, N)}{mid}
\end{equation}
\paragraph{Middle Price Move} It indicates the movement of middle price, which can simply be defined as the average of the current bid and ask prices being quoted.
\begin{equation}
    MiddleMove = \frac{mid}{\sum_{1 \leq t \leq T} \frac{1}{T}\left(shift(mid, t)\right)} - 1
\end{equation}
\paragraph{Buy-Sell Pressure} After getting enough data points, we can analyze the distribution of chips in the buying and selling direction.
\begin{equation}
    \begin{aligned}
        W^{buy}_i  &= \frac{1}{bp_1-mid} / \frac{1}{\sum_{1 \leq j \leq 5}(bp_j - mid)} \\
        W^{sell}_i &= \frac{1}{ap_1-mid} / \frac{1}{\sum_{1 \leq j \leq 5}(ap_j - mid)} \\
        P^{buy}    &= \sum_{1 \leq i \leq 5}\left(bv_i * W^{buy}_i\right) \\
        P^{sell}   &= \sum_{1 \leq i \leq 5}\left(av_i * W^{sell}_i\right)\\
        P &= \log (P^{buy}) - \log(P^{sell})
    \end{aligned}
\end{equation}
\paragraph{Weighted Price} The average price of ask and bid weighted by the corresponding volume.
\begin{equation}
    WP_i = \frac{av_i \cdot ap_i + bv_i \cdot bp_i}{av_i + bv_i}
\end{equation}
\paragraph{Order Imbalance} Order imbalance is a situation resulting from an excess of buy or sell orders for a specific security on a trading exchange, making it impossible to match the orders of buyers and sellers.
\begin{equation}
    QI_i = \frac{bv_i - av_i}{bv_i + av_i}
\end{equation}
\paragraph{Trend Strength} It describes the strength of the short-term trend.
\begin{equation}
    \begin{aligned}
        mid' &= mid - shift(mid, 1) \\    
        sum1 &= \sum_{t=1}^T shift(mid', t) \\
        sum2 &= \sum_{t=1}^T shift(|mid'|, t) \\
        TS   &= \frac{sum1}{sum2}
    \end{aligned}
\end{equation}

% \bibliographystyle{named}
% \bibliography{ijcai23}

% \small
% [40] G.-J. Qi, J. Tang, Z.-J. Zha, T.-S. Chua, and H.-J. 
% Zhang, “An efficient sparse metric learning in high-dimensional space via l 1-penalized log-determinant
% regularization,” in \textit{Proc. of ICML}, 2009.

% \small
% \noindent
% [41] Y. A. Malkov and D. A. Yashunin, “Efficient and robust approximate nearest neighbor search using hierarchical navigable small world graphs,” \textit{IEEE transactions on pattern analysis and machine intelligence},
% 2018.
